# Supplementary material for: A Survey on Open-Vocabulary Detection and Segmentation: Past, Present, and Future
Source: arXiv:2307.09220 source file (2024-04-15)
Supplement: Supplementary file 1 [file supplement.tex]

% \appendices  % DO NOT DELETE

% \section{Result Summary}
